# Supplementary material for: Domain Decomposition Method for the $N$-body Time-Independent and Time-Dependent Schr\"odinger Equation
Source: arXiv:1710.02401 source file (2017-10-06)
Supplement: Supplementary file 1 [file Appendix.tex]

\appendix{Antisymmetric wavefunction reconstruction}\label{APXA}
\noindent In order to construct an antisymmetric wavefunction, we propose a specific decomposition of $\R^{dN}$. Using the same notation as above, we first define:
\begin{definition}
 We denote by $\sigma(i;p,q) \in \{1,\cdots,L^{dN}\}$ the subdomain index such that, for $({\bf r}_1,\cdots,{\bf r}_p,\cdots,{\bf r}_q,\cdots,{\bf r}_N) \in \Omega_{i}$: $({\bf r}_1,\cdots,{\bf r}_q,\cdots,{\bf r}_p,\cdots,{\bf r}_N) \in \Omega_{\sigma(i;p,q)}$. Index $i$, refers to the subdomain index, and $(p,q)$ to the permutation coordinate indices.
\end{definition}
Notice that we naturally have $\sigma\big(\sigma(i;p,q);q,p\big)=i$. A priori, the basis functions $\big\{v_{j}^{iAp}\big\}_{1\leq j\leq K_i}$ in $\Omega_i$ and $\big\{v_{j}^{\sigma(i;p,q)}\big\}_{1\leq j\leq K_{\sigma(i;p,q)}}$ in $\Omega_{\sigma(i;p,q)}$ are distinct. Antisymmetry of the wavefunction would then occur, if and only if, for all $i \in\{1,\cdots,L^{dN}\}$, $\big\{v^{i}_j\big\}_{1\leq j\leq K_i}$ coincides with $\big\{v^{\sigma(i;p,q)}_j\big\}_{1\leq j \leq K_{\sigma(i;p,q)}}$, for all $(p,q) \in\{1,\cdots,N\}^2$.  We define
\begin{eqnarray*}
\Sigma(i)=\big\{\sigma(i;p,q)\in \{1,\cdots,L^{dN}\}, \, \forall (p,q)\in \{1,\cdots,N\}^2\big\}
\end{eqnarray*}
In order to guarantee the antisymmetry of the overall wavefunction, at any time, and any Schwarz iteration, the following fundamental {\it symmetry condition} must be full-filed. \\
\noindent{\it Symmetry condition}. For any $i\in \{1,\cdots,L^{dN}\}$ and for any $l \in \Sigma(i)$ the following condition holds. Say, for $l=\sigma(i;p,q)$, then
\begin{eqnarray}\label{FC}
\left.
\begin{array}{l}
\forall j \in \{1,\cdots,K_l\}, \,  \exists ! \widetilde{j} \in \{1,\cdots,K_i\}  \\
v^{l}_{j}({\bf r}_1,\cdots,{\bf r}_q,\cdots,{\bf r}_p,\cdots,{\bf r}_N) = v_{\widetilde{j}}^{i}({\bf r}_1,\cdots,{\bf r}_p,\cdots,{\bf r}_q,\cdots,{\bf r}_N) 
\end{array}
\right.
\end{eqnarray}
This is a non-trivial condition. In order to construct such a decomposition, we first introduce $\ell$ ``layers'' of $dN$-dimensional subdomains. Each layer $1\leq m \leq \ell$, which is denoted $\Xi_m \subset \R^{dN}$, is the union of $L_m$ subdomains, having all the same basis functions, and such that, for $m=1$ and $\lambda_1>0$
\begin{eqnarray}
\Xi_{1} = \big\{({\bf r}_1,\cdots,{\bf r}_N)\in \R^{dN} \, : \, |{\bf r}_i|_{\infty}\leq \lambda_1, \, \forall i \in \{1,\cdots,N\} \big\}
\end{eqnarray}
and for $m\geq 2$ and $\lambda_m>0$
\begin{eqnarray}
\Xi_{m} = \big\{({\bf r}_1,\cdots,{\bf r}_N)\in \R^{dN}  \, : \,  \lambda_{m-1}< |{\bf r}_i|_{\infty}\leq \lambda_m, \, \forall i \in \{1,\cdots,N\}  \big\}
\end{eqnarray}
where $|\cdot|_{\infty}$ denotes the $\ell^{\infty}(\R^d)$-norm. This decomposition ensures that, for any $1 \leq m \leq \ell$ with $\sum_{m=1}^{\ell}L_m=L^{dN}$,  and for any $(p,q) \in \{1,\cdots,N\}^2$,\\
 if $({\bf r}_1,\cdots,{\bf r}_p,\cdots,{\bf r}_q,\cdots,{\bf r}_N) \in \Xi_m$, then $({\bf r}_1,\cdots,{\bf r}_q,\cdots,{\bf r}_p,\cdots,{\bf r}_N) \in \Xi_m$, see Fig. \ref{ddm2}.
\begin{figure}[!ht]
\begin{center}
\hspace*{1mm}\includegraphics[height=8cm, keepaspectratio]{ddm2.eps}
\caption{Domain decomposition in layers ($\ell=3$) with $d=1$ and $N=2$.}
\label{ddm2}
\end{center}
\end{figure}
That is we define $\Xi_m$ as the following union: $\Xi_m=\cup_{l=m_-}^{m_+}\Omega_{l}$, of $m_+-m_-=L_m$ subdomains, having {\it all} the same basis wavefunctions, now denoted by $\big\{\hat{v}^1_{m},\cdots,\hat{v}_{m}^{K_m}\big\}$ where the upper index stands for the layer index. We have for $\Omega_i\subset \Xi_m$
\begin{eqnarray}\label{statWF}
\psi^{(k)}_i(\cdot,t) = \sum_{j=1}^{K_i}c_j^{i,(k)}(t)\hat{v}^i_{j}
\end{eqnarray}
 Then for any $\Omega_i \subset \Xi_{m}$, with $1 \leq m\leq \ell$, and $i \in \{m_-,\cdots,m_+\}$ we have:
\begin{eqnarray}\label{psi_tot}
\psi^{(k)}({\bf r}_1,\cdots,{\bf r}_N,t) = 
\left\{
\begin{array}{l}
\psi_i^{(k)}({\bf r}_1,\cdots,{\bf r}_N,t), \, ({\bf r}_1,\cdots,{\bf r}_N) \in \Omega_i-\omega_{i;j}, \, \forall (i,j) \in \{1,\cdots,L^{dN}\}^2\\
\\
\cfrac{\psi_i^{(k)}+\psi_j^{(k)}}{2}({\bf r}_1,\cdots,{\bf r}_N,t), \, ({\bf r}_1,\cdots,{\bf r}_N) \in \omega_{i;j}, \, \forall (i,j) \in \{1,\cdots,L^{dN}\}^2
\end{array}
\right.
\end{eqnarray}
We deduce by construction, the following proposition.
\begin{prop}
The wavefunction $\psi^{(k)}$, defined in \eqref{statWF} and \eqref{psi_tot} is antisymmetric.
\end{prop} 
\noindent{\bf Proof.} We consider 4 different cases. 
\begin{itemize}
\item First, for any $({\bf r}_1,\cdots,{\bf r}_p,\cdots,{\bf r}_q,\cdots,{\bf r}_N) \in \Omega_i-\omega_{i;j} \subset \Xi_m$, for some $1 \leq m \leq \ell$, we have $({\bf r}_1,\cdots,{\bf r}_p,\cdots,{\bf r}_q,\cdots,{\bf r}_N) \in \Xi_m$, then 
\begin{eqnarray*}
\left.
\begin{array}{lcl}
\psi^{(k)}({\bf r}_1,\cdots,{\bf r}_p, \cdots,{\bf r}_q,\cdots, {\bf r}_N,t) & =& \psi_i^{(k)}({\bf r}_1,\cdots,{\bf r}_p, \cdots,{\bf r}_q,\cdots, {\bf r}_N,t)\\
\\
&  = & -\psi_i^{(k)}({\bf r}_1,\cdots,{\bf r}_q, \cdots,{\bf r}_p,\cdots, {\bf r}_N,t)\\
\\
&  =&  -\psi^{(k)}({\bf r}_1,\cdots,{\bf r}_q, \cdots,{\bf r}_p,\cdots, {\bf r}_N,t)
\end{array}
\right.
\end{eqnarray*}
\item Secondly, for $({\bf r}_1,\cdots,{\bf r}_p,\cdots,{\bf r}_q,\cdots,{\bf r}_N) \in \omega_{i;j} \subset \Xi_m$, such that $\Omega_j \subset \Xi_m$, the antisymmetry condition is still satisfied, as $\Omega_j$ has the same basis function as $\Omega_i$. \\
Thirdly, for $({\bf r}_1,\cdots,{\bf r}_p,\cdots,{\bf r}_q,\cdots,{\bf r}_N) \in \omega_{i;j} \subset \Xi_m$ with $j$ unique, such that $\Omega_j \not \subset \Xi_m$. Then there exists a (unique) $p \in \{1,\cdots,\ell\}$ such that $\Omega_j \subset \Xi_p$, \\
that is $({\bf r}_1,\cdots,{\bf r}_p,\cdots,{\bf r}_q,\cdots,{\bf r}_N) \in \Xi_m \cap \Xi_p$. By construction \\
$({\bf r}_1,\cdots,{\bf r}_q,\cdots,{\bf r}_p,\cdots,{\bf r}_N) \in \Xi_m \cap \Xi_p$ which ensures that we also have
\begin{eqnarray*}
\left.
\begin{array}{lcl}
\psi^{(k)}({\bf r}_1,\cdots,{\bf r}_N,t) & = &\cfrac{\psi_i^{(k)}+\psi_j^{(k)}}{2}({\bf r}_1,\cdots,{\bf r}_N,t)\\
& & \hbox{for } \, ({\bf r}_1,\cdots,{\bf r}_N) \in \Xi_m\cap\Xi_p
\end{array}
\right.
\end{eqnarray*}
We then have
\begin{eqnarray*}
\left.
\begin{array}{lcl}
\psi^{(k)}({\bf r}_1,\cdots,{\bf r}_q,\cdots,{\bf r}_p,\cdots,{\bf r}_N,t) & = &\cfrac{\psi_i^{(k)}+\psi_j^{(k)}}{2}({\bf r}_1,\cdots,{\bf r}_q,\cdots,{\bf r}_p,\cdots,{\bf r}_N,t)\\
& =& -\cfrac{\psi_i^{(k)}}{2}({\bf r}_1,\cdots,{\bf r}_q,\cdots,{\bf r}_p,\cdots,{\bf r}_N,t)\\
& & -\cfrac{\psi_j^{(k)}}{2}({\bf r}_1,\cdots,{\bf r}_p,\cdots,{\bf r}_q,\cdots,{\bf r}_N,t) \\
& = & -\cfrac{\psi_i^{(k)}+\psi_j^{(k)}}{2}({\bf r}_1,\cdots,{\bf r}_p,\cdots,{\bf r}_q,\cdots,{\bf r}_N,t)\\
\\
& = & -\psi^{(k)}({\bf r}_1,\cdots,{\bf r}_p,\cdots,{\bf r}_q,\cdots,{\bf r}_N,t)\\
\\
& & \hbox{for } \,  ({\bf r}_1,\cdots,{\bf r}_q,\cdots,{\bf r}_p,\cdots,{\bf r}_N) \in \Xi_m\cap\Xi_p
\end{array}
\right.
\end{eqnarray*}
\item The fourth and last case occurs when for $({\bf r}_1,\cdots,{\bf r}_p,\cdots,{\bf r}_q,\cdots,{\bf r}_N)\in \widetilde{\omega}_i$, that is \\
$({\bf r}_1,\cdots,{\bf r}_p,\cdots,{\bf r}_q,\cdots,{\bf r}_N) \in \omega_{i;i_j} \subset \Xi_m$, with $j \in \{1,\cdots,\mathcal{O}(\widetilde{\omega}_i)\}$ and such that $\Omega_{i_j} \subset \Xi_p$ or $\Omega_{i_j} \not \subset \Xi_m$, with $1\leq j \leq \mathcal{O}(\widetilde{\omega}_i)$. Then there still exists a (unique) $p \in \{1,\cdots,\ell\}$ such that $\Omega_{i_j} \subset \Xi_p$, such that $({\bf r}_1,\cdots,{\bf r}_p,\cdots,{\bf r}_q,\cdots,{\bf r}_N) \in \Xi_m \cap \Xi_p$. \\
This situation occurs when $({\bf r}_1,\cdots,{\bf r}_p,\cdots,{\bf r}_q,\cdots,{\bf r}_N)$ belongs to more than $2$ subdomains; more specifically up to $2^{dN}$ subdomains, including of course $\Omega_i$. However these subdomains belong to either $\Xi_m$ or $\Xi_p$. As a consequence the arguments used in the third situation is still valid, except that we this time have to average the wavefunction as follows: for $({\bf r}_1,\cdots,{\bf r}_q,\cdots,{\bf r}_p,\cdots,{\bf r}_N) \in \Xi_m \cap \Xi_{p}$ which ensures that we also have
\begin{eqnarray*}
\left.
\begin{array}{l}
\psi^{(k)}({\bf r}_1,\cdots,{\bf r}_N,t)  = \cfrac{1}{\textrm{Card}\mathcal{O}(\widetilde{\omega}_i)+1}\big(\psi_i^{(k)}+\sum_{j=1}^{\mathcal{O}(\widetilde{\omega}_i)}\psi_{i_j}^{(k)}\big)({\bf r}_1,\cdots,{\bf r}_N,t) \,\\
  \hbox{ for } \, ({\bf r}_1,\cdots,{\bf r}_N) \in \Xi_m\cap\Xi_p
\end{array}
\right.
\end{eqnarray*}
We again use the local antisymmetry to conclude. 
\end{itemize}
This conclude the proof. $\Box$\\
\\
\noindent The decomposition 
\begin{eqnarray*}
\R^{dN} = \cup_{m=1}^{\ell}\Xi_m = \cup_{m=1}^{\ell}\big(\cup_{i=m_-}^{m_+}\Omega_i\big)
\end{eqnarray*}
is somehow restrictive, as it requires identical basis functions, in any subdomain contained in a given $\Xi_m$, but this last conditions is also quite reasonable if we locate the nuclei at the center of $\cup_{m=1}^{\ell}\Xi_m$. Domain decomposition in 2-D is summarized in Fig. \ref{ddm_over}.
\begin{figure}[!ht]
\begin{center}
\hspace*{1mm}\includegraphics[height=8cm, keepaspectratio]{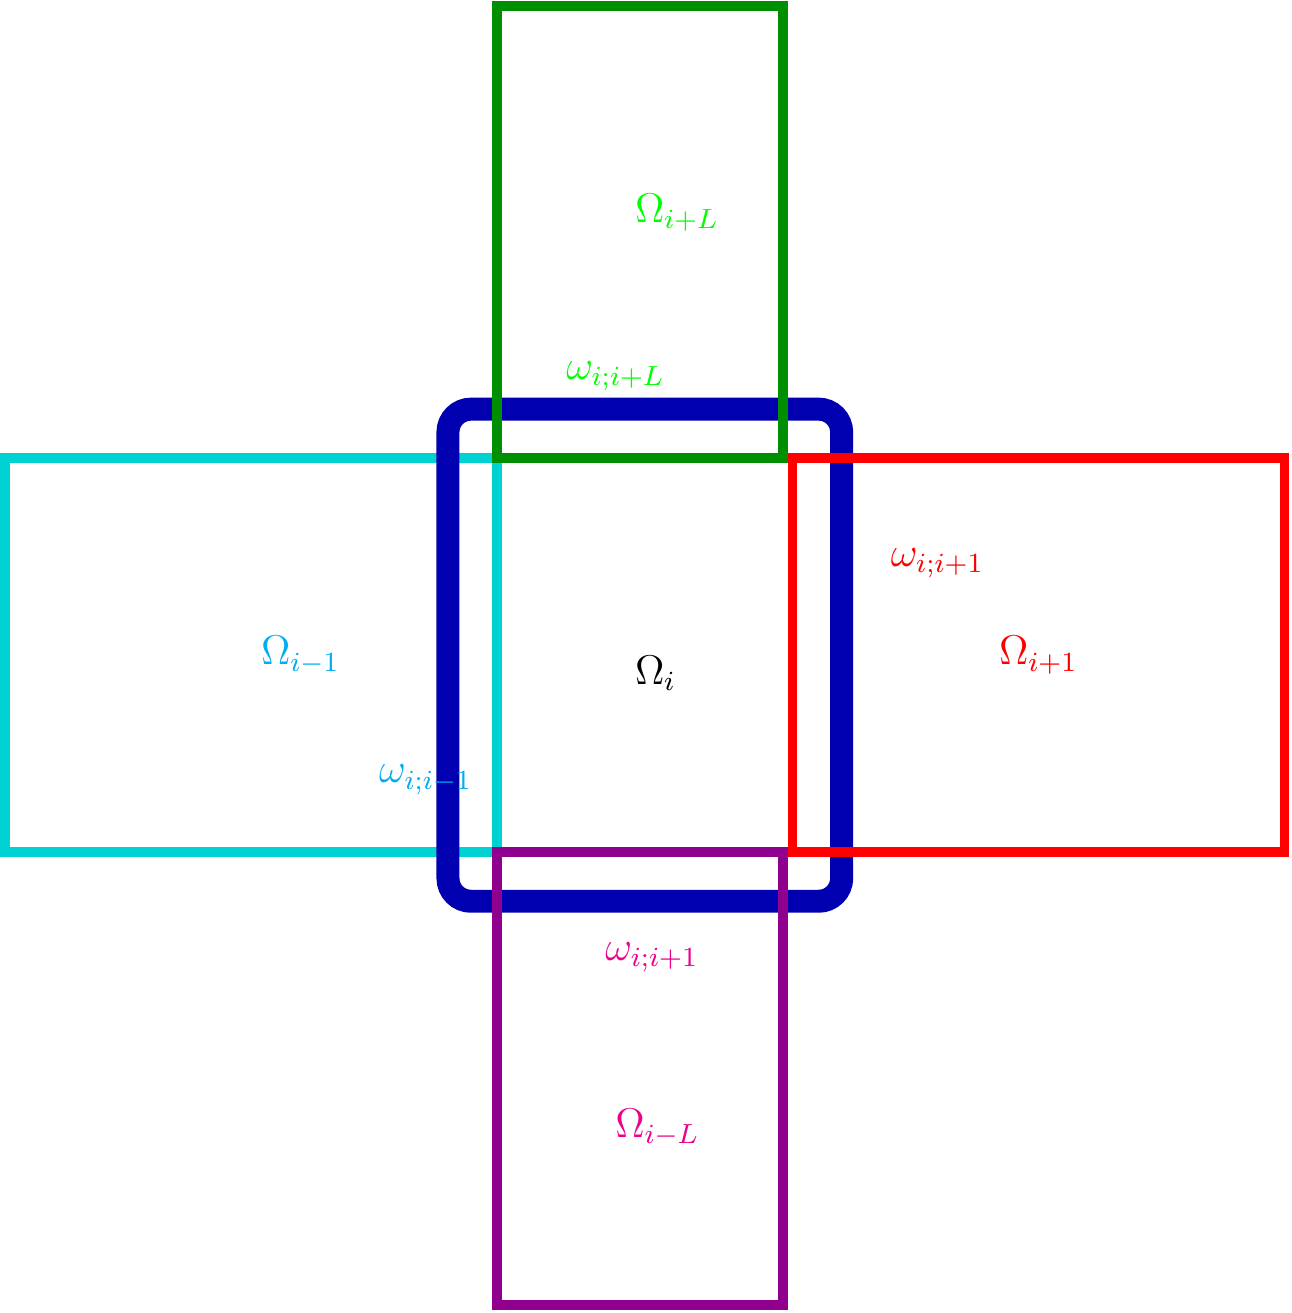}
\caption{Domain decomposition with overlapping region on $\Omega_i$ with $\Omega_{j,k,l,m}$ in $\R^2$}
\label{ddm_over}
\end{center}
\end{figure}
